# Supplementary material for: AEGIS: Runtime-Guided GPU Collocation for Multi-Tenant Deep Learning Training
Source: arXiv:2508.19073 source file (2026-10-06)
Supplement: Supplementary file 1 [file 10-appendix.tex]

\onecolumn
\section{Appendix}
\label{appendix}

\subsection{Artifacts}
